# Supplementary material for: On Forgetting and Stability of Score-based Generative models
Source: arXiv:2601.21868 source file (2026-06-02)
Supplement: Supplementary file 1 [file 10_mixture_calculations.tex]

\section{Explicit constant for mixtures}
In this section, we consider for given sequences $i \in \nset \rightarrow \mixtcoeff{i} \in \rset^{\xdim}$, $i \in \nset \rightarrow \mixtcovar{i}{0} \in \msetpos{\rset^\xdim}$ and
$i \in \nset \rightarrow \mixtcoeff{i}$ such that $\sum_i \mixtcoeff{i} = 1$ the distribution 
\begin{equation}
    \label{eq:def:pdatamixture}
    \pdata \eqdef \sum_{i \in \nset} \mixtcoeff{i} \gaussiand{\mixtmean{i}}{\mixtcovar{i}{0}} \eqsp.
\end{equation}
It is then easy to see that$ \fwdmarg{t} = \sum_{i \in \nset} \mixtcoeff{i} \gaussiand{\mixtmean{i}}{\mixtcovar{i}{t}}$,
with $\mixtcovar{i}{t} \eqdef \mixtcovar{i}{0} + \fwdvar{0}{t} \Id$ and that
\begin{equation}
    \bwdker{t}[0][\x][\set{A}] = \sum_{i \in \nset} \bwdmixtcoeff{i}{t}{0}{x} \int \indi{A}{\x_0} \gaussiand{\bwdmixtmean{i}{t}{0}{\x}}{\bwdmixtcovar{i}{t}{0}}[\x_0] \rmd \x_0 \eqsp,
\end{equation}
with $\bwdmixtcovar{i}{t}{0} \eqdef \fwdvar{0}{t}\mixtcovar{i}{0}\mixtcovar{i}{t}^{-1}$, $\bwdmixtmean{i}{t}{0}{\x} \eqdef \mixtcovar{i}{0}\left(\mixtcovar{i}{t}^{-1}(\x - \mixtmean{i}) + \mixtcovar{i}{0}^{-1}\mixtmean{i}\right)$ and
\begin{equation}
    \bwdmixtcoeff{i}{t}{0}{\x} \eqdef \frac{\mixtcoeff{i}\gaussiand{\mixtmean{i}}{\mixtcovar{i}{t}}[\x]}{\sum_{j \in \nset} \mixtcoeff{j}\gaussiand{\mixtmean{j}}{\mixtcovar{j}{t}}[\x]} \eqsp.
\end{equation}
Young's inequality implies that for any $\zeta \in \rset$,
\begin{align}
    \normMH{\x_0 - \bwdmixtmean{i}{t}{0}{\x}}{\bwdmixtcovar{i}{t}{0}}^2 
    \leq \left(1 + \zeta^2\right)\normMH{\x_0 - \mixtmean{i}}{\bwdmixtcovar{i}{t}{0}^{-1}}^2 
    + \left(1 + \zeta^{-2}\right)\normMH{\x - \mixtmean{i}}{\bwdmixtcovar{i}{t}{0}^{-1}}^2
\end{align}
which leads to the lower bound
\begin{equation*}
    \gaussiand{\bwdmixtmean{i}{t}{0}{\x}}{\bwdmixtcovar{i}{t}{0}}[\x_0] \geq \frac{1}{(1 + \zeta^2)^{\xdim}}\gaussiand{\mixtmean{i}}{(1 + \zeta^2)^{-1}\bwdmixtcovar{i}{t}{0}}[\x_0] \exp\left(-\frac{1 + \zeta^{-2}}{2}\normMH{\x - \mixtmean{i}}{\bwdmixtcovar{i}{t}{0}^{-1}}^2\right)\eqsp.
\end{equation*}
We now seek a lower bound of
\begin{align*}
    &\bwdmixtcoeff{i}{t}{0}{\x}\exp\left(-\frac{1 + \zeta^{-2}}{2}\normMH{\x - \mixtmean{i}}{\bwdmixtcovar{i}{t}{0}^{-1}}^2\right) \\
    &= \left[\sum_{j \in \nset}\exp\left(\frac{1}{2}\left[(1+\zeta^{-2})\normMH{\x - \mixtmean{i}}{\bwdmixtcovar{i}{t}{0}^{-1}}^2 + \normMH{\x-\mixtmean{i}}{\mixtcovar{i}{t}^{-1}}^2 - \normMH{\x-\mixtmean{j}}{\mixtcovar{j}{t}^{-1}}^2\right] + \log\left(\frac{\mixtcoeff{j}}{\mixtcoeff{i}}\right) + \frac{\xdim}{2}\log\left(\frac{\det{\mixtcovar{i}{t}}}{\det{\mixtcovar{j}{t}}}\right)\right) \right]^{-1} \\
    &=\left[\sum_{j \in \nset}\exp\left(\frac{1}{2}\left[\frac{(1+\zeta^{-2})}{\fwdvar{0}{t}}\normMH{\mixtcovar{i}{0}^{1/2}\left(\x - \mixtmean{i}\right)}{\mixtcovar{i}{t}^{-1}}^2 + \normMH{\x-\mixtmean{i}}{\mixtcovar{i}{t}^{-1}}^2 - \normMH{\x-\mixtmean{j}}{\mixtcovar{j}{t}^{-1}}^2\right] + \log\left(\frac{\mixtcoeff{j}}{\mixtcoeff{i}}\right) + \frac{\xdim}{2}\log\left(\frac{\det{\mixtcovar{i}{t}}}{\det{\mixtcovar{j}{t}}}\right)\right) \right]^{-1}\eqsp.
\end{align*}
for $\x \in \convexhull{\{\mixtmean{i}\}_{i \in \nset}}$.
If we let 
\begin{equation*}
    a_{k, i}(\x) \eqdef \frac{1}{2}\left[\frac{(1+\zeta^{-2})}{\fwdvar{0}{t}}\normMH{\mixtcovar{i}{0}^{1/2}\left(\x - \mixtmean{i}\right)}{\mixtcovar{i}{t}^{-1}}^2 + \normMH{\x-\mixtmean{i}}{\mixtcovar{i}{t}^{-1}}^2 - \normMH{\x-\mixtmean{j}}{\mixtcovar{j}{t}^{-1}}^2\right] + \log\left(\frac{\mixtcoeff{j}}{\mixtcoeff{i}}\right) + \frac{\xdim}{2}\log\left(\frac{\det{\mixtcovar{i}{t}}}{\det{\mixtcovar{j}{t}}}\right) \eqsp,
\end{equation*}
and $\logsumexp{\omega_k}{k \in \nset} = \log \left(\sum_{k \in \nset} \exp(\omega_k)\right)$, then we have that
\begin{equation*}
    \bwdmixtcoeff{i}{t}{0}{\x}\exp\left(-\frac{1 + \zeta^{-2}}{2}\normMH{\x - \mixtmean{i}}{\bwdmixtcovar{i}{t}{0}^{-1}}^2\right) = \exp\left(-\logsumexp{a_{k, i}(\x)}{k \in \nset}\right)\eqsp.
\end{equation*}
Therefore, finding the lower bound amounts to finding the maximum of the function
\begin{equation*}
    \logsumexp{a_{k, i}(\x)}{k \in \nset}
\end{equation*}
for $\x \in \convexhull{\{\mixtmean{i}\}_{i \in \nset}}$. Note that $\logsumexp{}{}$ is a convex function, thus as long as we can assure that each $a_{k, i}(\x)$ is a convex function on $\x \in \convexhull{\{\mixtmean{i}\}_{i \in \nset}}$, we will know that the maximum is on the boundaries of the domain.

Note that for all $k, i$, 
\begin{equation*}
    \nabla^2a_{k, i}(\x) = \frac{1}{2}\left[(1 + \zeta^{-2})\bwdmixtcovar{i}{t}{0}^{-1} + \mixtcovar{i}{t}^{-1} - \mixtcovar{k}{t}^{-1}\right] \eqsp.
\end{equation*}
Thus, $a_{k, i}$ is convex if and only if
\begin{align*}
    &\mixtcovar{k}{t}^{-1} \leq (1 + \zeta^{-2})\bwdmixtcovar{i}{t}{0}^{-1} + \mixtcovar{i}{t}^{-1} = \frac{1 + \zeta^{-2}}{\fwdvar{0}{t}}\mixtcovar{i}{t}^{-1} \mixtcovar{i}{0} + \mixtcovar{i}{t}^{-1} \\
    &=\frac{1 + \zeta^{-2}}{\fwdvar{0}{t}}\mixtcovar{i}{t}^{-1}\left(\mixtcovar{i}{0} + \Id\right) 
\end{align*}
It is therefore enough to chose $\zeta^{-2}$ such that for every $k, i$
\begin{equation}
    \frac{1 + \zeta^{-2}}{\fwdvar{0}{t}} \geq \operatorname{eigmax}\left(\mixtcovar{k}{t}^{-1}\left(\mixtcovar{i}{0} + \Id\right)^{-1}\mixtcovar{i}{t}\right) 
\end{equation}
In particular, considering $\mixtcovar{i}{0} = \eta_i^2 \Id$
we get that it is enough to have
\begin{equation}
    \zeta^{-2} \geq \fwdvar{0}{t}\frac{\eta_i^2 + \fwdvar{0}{t}}{(\eta_k^2  + \fwdvar{0}{t})(\eta_i^2 + 1)} - 1  = \eqsp.
\end{equation}
